# Supplementary material for: OmniLocalRF: Omnidirectional Local Radiance Fields from Dynamic Videos
Source: arXiv:2404.00676 source file (2024-03-31)
Supplement: Supplementary file 1 [file OmniLocalRF-supple.tex]

%\documentclass[10pt,twocolumn,letterpaper]{article}
\documentclass[OmniLocalRF-main.tex]{subfiles}

\usepackage{cvpr}              %


\input{mypackages}
\definecolor{cvprblue}{rgb}{0.21,0.49,0.74}
\usepackage[pagebackref,breaklinks,colorlinks,citecolor=cvprblue]{hyperref}

\def\paperID{3021} %
\def\confName{CVPR}
\def\confYear{2024}

\input{title}
\setcounter{page}{1}

\input{authors}

\begin{document}
\maketitlesupplementary

\input{sec/supple}

{
    \small
    \bibliographystyle{ieeenat_fullname}
    \bibliography{OmniLocalRF-reference}
}


\end{document}
